# Supplementary material for: Stochastic Unrolled Federated Learning
Source: arXiv:2305.15371 source file (2024-02-06)
Supplement: Supplementary file 1 [file Constrained_Appendix.tex]

\section{Training via Constrained Learning}
In this section, we demonstrate the mechanism of solving the constrained problem \eqref{eq:surf} in the dual domain through the constrained learning theory (CLT). The main idea is to construct the dual problem of \eqref{eq:surf}, which converts it into an unconstrained problem with the help of a set of dual variables $\lambda_{l}$ for all $l$. Solving the dual problem is then doable using Algorithm \ref{alg:PD}.

To be more precise, the dual problem of \eqref{eq:surf} is equivalent to finding the saddle point of the Lagrangian function 
\begin{equation}\label{eq:statlagrang}
    \begin{split}
        {\cal L}(\boldsymbol{\theta}, {\boldsymbol \lambda}) =  \mathbb{E} \big[{f}(\boldsymbol{\Phi}({\boldsymbol{\vartheta}}; \boldsymbol{\theta})) \big]
        + 
        \sum_{l=1}^L &{\lambda}_{l} \mathbb{E} \Big[\mathbb{E} \big[ \| \nabla f({\bf W}_{l})\|\ | \ {\cal F}_{l-1} \big] - (1-\epsilon) \ \|  \nabla f({\bf W}_{l-1}) \|  \Big],\\
        % &+ \Big.
        % {\nu}_{i,l} \cdot 
        % \mathbb{E}\left[\|\widehat{\bf y}_{i,l-1} - {\bf y}_i^*\|  -  \|\widehat{\bf y}_{i,l} - {\bf y}_i^*\|  - \epsilon \|{\bf y}_i^*\|  \right] \Big),
    \end{split}
\end{equation}
where ${\boldsymbol \lambda} \in {\mathbb{R}^{L}_+}$ is a vector collecting the dual variables $\lambda_{l}$. Since the expectation is with respect to an unknown distribution, we resort to the empirical version of the Lagrangian function
\begin{equation}\label{eq:emplagrang}
    \begin{split}
        \widehat{\cal L}(\boldsymbol{\theta}, {\boldsymbol \lambda}) =  \widehat{\mathbb{E}} \big[{f}(\boldsymbol{\Phi}({\boldsymbol{\vartheta}}; \boldsymbol{\theta})) \big]
        + 
        \sum_{l=1}^L &{\lambda}_{l} \widehat{\mathbb{E}} \Big[\widehat{\mathbb{E}} \big[ \| \nabla f({\bf W}_{l})\|\ | \ {\cal F}_{l-1} \big] - (1-\epsilon) \ \|  \nabla f({\bf W}_{l-1}) \|  \Big],
    \end{split}
\end{equation}
where $\widehat{\mathbb{E}}$ denotes the sample mean evaluated over $Q$ realizations. The empirical dual problem can then be cast as 
\begin{equation}\label{eq:dual}
    \begin{split}
        \widehat{D}^* = \max_{{\boldsymbol \lambda} \in \mathbb{R}^{L}_+} \ \min_{\boldsymbol{\theta}\in \mathbb{R}^p} \ \widehat{\cal L}(\boldsymbol{\theta}, {\boldsymbol \lambda}).
    \end{split}
\end{equation}
Equation \eqref{eq:dual} is an unconstrained optimization problem that is not harder than an empirical risk minimization (ERM) problem. That is the case since the inner minimization for a fixed $\boldsymbol{\lambda}$ is akin to an ERM problem with a regularization term. Moreover, the dual function is a pointwise minimum of a family of affine functions and therefore is concave by definition, which makes the outer maximization doable. 

Nevertheless, \eqref{eq:dual} is not equivalent to \eqref{eq:surf} due to the non-convexity of the problem and the empirical gap induced by replacing the statistical expectations with empirical ones. A precise characterization of the gap between the two problems is provided by CLT. 
\begin{theorem}[CLT]\label{thm:CLT}
Let $P^*$ be the optimal value of \eqref{eq:surf} and $(\boldsymbol{\theta}^*, \boldsymbol{\lambda}^*)$ be a stationary point of \eqref{eq:dual}. Under Assumptions \ref{A1}- \ref{A5}, it holds, for some constant $\rho$, that 
\begin{equation}\label{eq:nearOptimal}
    |P^* - \widehat{D}^*| \leq M \nu + \rho \ \zeta(Q, \delta), \ \text{and}
\end{equation} 
\begin{equation}\label{eq:constraints}
    \begin{split}
         \mathbb{E} \Big[\mathbb{E} \big[ \| \nabla f({\bf W}_{l})\|\ | \ {\cal F}_{l-1} \big] - (1-\epsilon) \ \|  \nabla f({\bf W}_{l-1}) \|  \Big] \leq \zeta(Q, \delta), \quad  \forall l,
    \end{split}
\end{equation}
with probability $1-\delta$ each and with $\rho \geq \max \{ \| \boldsymbol{\lambda}^*\|, \| \overline{\boldsymbol{\lambda}}^* \| \}$, where $\overline{\boldsymbol{\lambda}}^* = \textup{argmax}_{{\boldsymbol \lambda}} \ \min_{\boldsymbol{\theta}} \ {\cal L}(\boldsymbol{\theta}, {\boldsymbol \lambda})$.
\end{theorem}
The proof of this theorem goes along the lines of the proofs in \citep{chamon2022constrained}.

CLT, therefore, suggests that solving \eqref{eq:dual} generates probably approximately correct solutions to \eqref{eq:surf}. Moreover, the optimality and feasibility of these solutions are controlled by a few factors: the Lipschitz constant $M$ as per Assumption \ref{A1}; the richness parameter $\nu$ of the parameterization $\boldsymbol{\theta}$ as per Assumption \ref{A3}; the sample size (see Assumption \ref{A2}); and the sensitivity to the constraints embodied with the dual variables. 

While CLT shows that a probably approximately correct solution exists, it does not provide a mechanism to find this solution. Finding this solution is, as we mentioned earlier, possible by alternating between minimizing $\widehat{\cal L}$ with respect to $\boldsymbol{\theta}$ for a fixed $\boldsymbol{\lambda}$ and then updating the latter using the minimizer. This process is described in detail in Algorithm \ref{alg:PD}.

\begin{algorithm}
\caption{Primal-Dual Training Algorithm}\label{alg:PD}
\begin{algorithmic}[1]
 \State {\bfseries Input:} Meta-training dataset ${\bf D} = \{\boldsymbol{\vartheta}_m \}_{m=1}^{M}$.
 \State Initialize $\boldsymbol{\theta} =\{\boldsymbol{\theta}_l\}_{l=1}^L$ and ${\boldsymbol \lambda} = \{ {\boldsymbol \lambda}_{l} \}_{l=1}^L$.
\For{each epoch}
    \For{each batch}
    \State Sample a dataset from ${\bf D}$.
    \State Compute $\widehat{\cal L}(\boldsymbol{\theta}, {\boldsymbol \lambda})$ as in \eqref{eq:emplagrang}.
    \For{$l = 1, \dots, L$}
    \State Update variables at layer $l$:
    \begin{align}
        \boldsymbol{\theta}_l &\gets [\boldsymbol{\theta}_l - \mu_{\theta} \nabla_{\boldsymbol{\theta}_l} \widehat{\cal L}(\boldsymbol{\theta}, {\boldsymbol \lambda})], \label{eq:ADAM}\\
        {\boldsymbol \lambda}_{l} & \gets [{\boldsymbol \lambda}_{l} + \mu_{\lambda} \nabla_{{\boldsymbol \lambda}_{l}} \widehat{\cal L}(\boldsymbol{\theta}, {\boldsymbol \lambda})]_+.\label{eq:lr_dual}
    \end{align}
    
    % \begin{equation}\label{eq:ADAM}
        
    % \end{equation}
    % \begin{equation}\label{eq:lr_dual}
    % \begin{split}
        
    % \end{split}
% \end{equation}
\EndFor
\EndFor
\EndFor
 \State {\bfseries Return:} $\boldsymbol{\theta}_l^* \gets \boldsymbol{\theta}_l, \forall l\in\{1, \dots, L\}$.
\end{algorithmic}
\end{algorithm}
